# Supplementary material for: Development of Zero-Noise Extrapolated Projection Based Quantum Algorithm for Accurate Evaluation of Molecular Energetics in Noisy Quantum Devices
Source: arXiv:2306.14560 ancillary file (2023-06-26)
Supplement: Supplementary file 1 [file Supplementary_Material.pdf]

# Supplementary Material for “Development of Zero-Noise Extrapolated Projection Based Quantum Algorithm for Accurate Evaluation of Molecular Energetics in Noisy Quantum Devices”

Chinmay Shrikhande, Sonaldeep Halder, and Rahul Maitra

| Qubit | T1 (us) | T2 (us) | Frequency (GHz) |
|---|---|---|---|
| 0 | 185.254566672058 | 108.590561787158 | 4.96229035100335 |
| 1 | 268.579638691792 | 76.274293361891 | 4.83786796591827 |
| 2 | 187.442161803573 | 22.6443570304886 | 5.03725027235381 |
| 3 | 174.737706167419 | 61.0145706272333 | 4.95096136960501 |
| 4 | 90.5841434627008 | 44.9021694062365 | 5.06512727546072 |

| Prob meas1 prep0 | Readout length (ns) | ID error | √x (sx) error |
|---|---|---|---|
| 0.0122 | 5351.11111111111 | 0.000213047113239 | 0.000213047113239 |
| 0.0076 | 5351.11111111111 | 0.000196040957688 | 0.000196040957688 |
| 0.01 | 5351.11111111111 | 0.000294533234303 | 0.000294533234303 |
| 0.0114 | 5351.11111111111 | 0.000269493743071 | 0.000269493743071 |
| 0.0076 | 5351.11111111111 | 0.000378852015259 | 0.000378852015259 |

| Anharmonicity (GHz) | Readout assignment error | Prob meas0 prep1 |
|---|---|---|
| -0.344625413538411 | 0.024 | 0.0358 |
| -0.345283846738963 | 0.0155 | 0.0234 |
| -0.342551284436791 | 0.0256 | 0.0412 |
| -0.343578390756953 | 0.0179 | 0.0244 |
| -0.342107638982877 | 0.0177 | 0.0278 |

| Pauli-X error | CNOT error | Gate time (ns) |
|---|---|---|
| 0.000213047113239 | 0_1:0.0061374126725864675 | 0_1:277.333333333333 |
| 0.000196040957688 | 1_2:0.011721515540077776 | 1_0:0.0061374126725864675 |
| 0.000294533234303 | 2_3:0.006814063171862034 | 2_1:0.011721515540077776 |
| 0.000269493743071 | 3_4:0.006881247976205179 | 3_2:0.006814063171862034 |
| 0.000378852015259 | 4_3:0.006881247976205179 | 4_3:298.666666666663 |

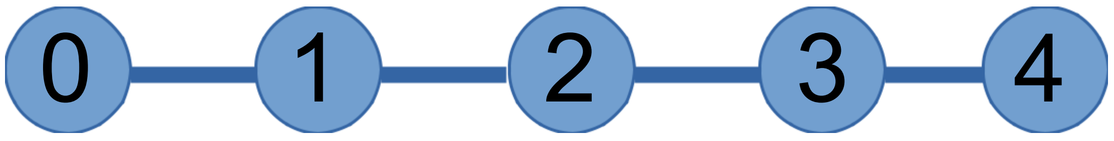


Figure S1. Properties and connectivity for IBM’s superconducting quantum device *ibmq_manila*

| Qubit | T1 (us) | T2 (us) | Frequency (GHz) |
|---|---|---|---|
| 0 | 134.104197000105 | 138.784424633589 | 5.09021453277135 |
| 1 | 92.4182861367789 | 105.918891345344 | 5.24552989408971 |
| 2 | 117.505079949194 | 63.9338952671585 | 5.36149792044671 |
| 3 | 47.0421480391281 | 122.873315457405 | 5.17031956046109 |
| 4 | 82.9974486905277 | 147.729664965997 | 5.25846674570156 |

| Prob meas1 prep0 | Readout length (ns) | ID error | √x (sx) error |
|---|---|---|---|
| 0.0068 | 6158.22222222222 | 0.000173125759261 | 0.000173125759261 |
| 0.0064 | 6158.22222222222 | 0.000256462528433 | 0.000256462528433 |
| 0.0058 | 6158.22222222222 | 0.000234889110331 | 0.000234889110331 |
| 0.0116 | 6158.22222222222 | 0.000247157734351 | 0.000247157734351 |
| 0.0076 | 6158.22222222222 | 0.000267214238156 | 0.000267214238156 |

| Anharmonicity (GHz) | Readout assignment error | Prob meas0 prep1 |
|---|---|---|
| -0.336123005182165 | 0.0207 | 0.0346 |
| -0.316572131412737 | 0.0211 | 0.0358 |
| -0.330627488458493 | 0.0234 | 0.041 |
| -0.33739226113681 | 0.0193 | 0.027 |
| -0.331345143237128 | 0.0207 | 0.0338 |

| Pauli-X error | CNOT error | Gate time (ns) |
|---|---|---|
| 0.000173125759261 | 0_1:0.0126847265271522 46 | 0_1:810.666666666666 |
| 0.000256462528433 | 1_3:0.00658361641185814 5 | 1_2:0.00622434237816862 9 |
| 0.000234889110331 | 2_1:0.00622434237816862 9 | 2_1:384 |
| 0.000247157734351 | 3_4:0.00751511837389934 3 | 3_1:0.00658361641185814 5 |
| 0.000267214238156 | 4_3:0.00751511837389934 3 | 4_3:490.666666666663 |

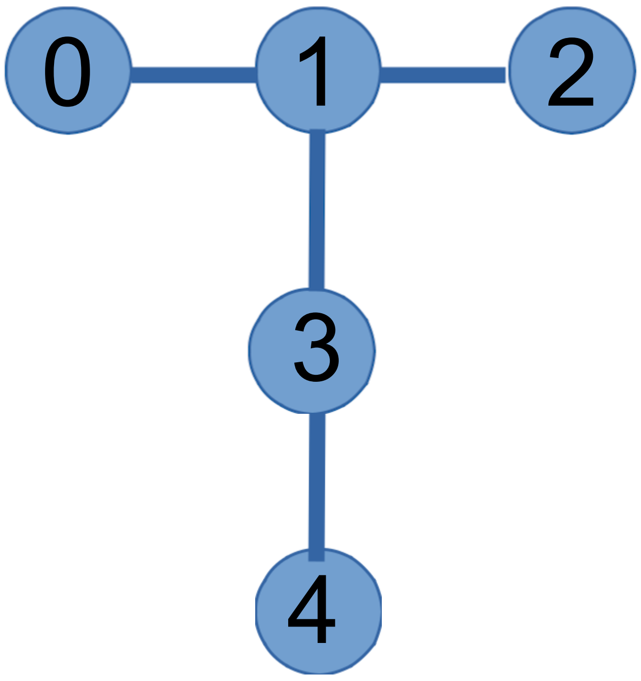


Figure S2. Properties and connectivity for IBM's superconducting quantum device *ibmq_belem*
